# Supplementary material for: Population-informed priors in gravitational-wave astronomy
Source: arXiv:2108.02462 ancillary file (2021-11-10)

# SUPPLEMENTAL MATERIAL

## Population-informed priors in gravitational-wave astronomy

Christopher J. Moore<sup>1,\*</sup> and Davide Gerosa<sup>1,2,3</sup>

<sup>1</sup>*Institute for Gravitational Wave Astronomy & School of Physics and Astronomy, University of Birmingham, Edgbaston, Birmingham B15 2TT, UK*

<sup>2</sup>*Dipartimento di Fisica “G. Occhialini”, Università degli Studi di Milano-Bicocca, Piazza della Scienza 3, 20126 Milano, Italy*

<sup>3</sup>*INFN, Sezione di Milano-Bicocca, Piazza della Scienza 3, 20126 Milano, Italy*

We provide 2D projections in the  $(m_1, m_2)$  (left column),  $(\chi_1, \chi_2)$  (middle column)  $(\cos \theta_1, \cos \theta_2)$  (right column) parameter spaces for all the event in the 44 gravitational-wave events considered (top to bottom). As in the main body of the paper, blue, red, and green curves refer to the uninformative, hierarchical, and empirical estimate of the posterior, respectively. In the joint 2D panels we show 50% confidence intervals. The event labels in the left panels refer to the entire row.

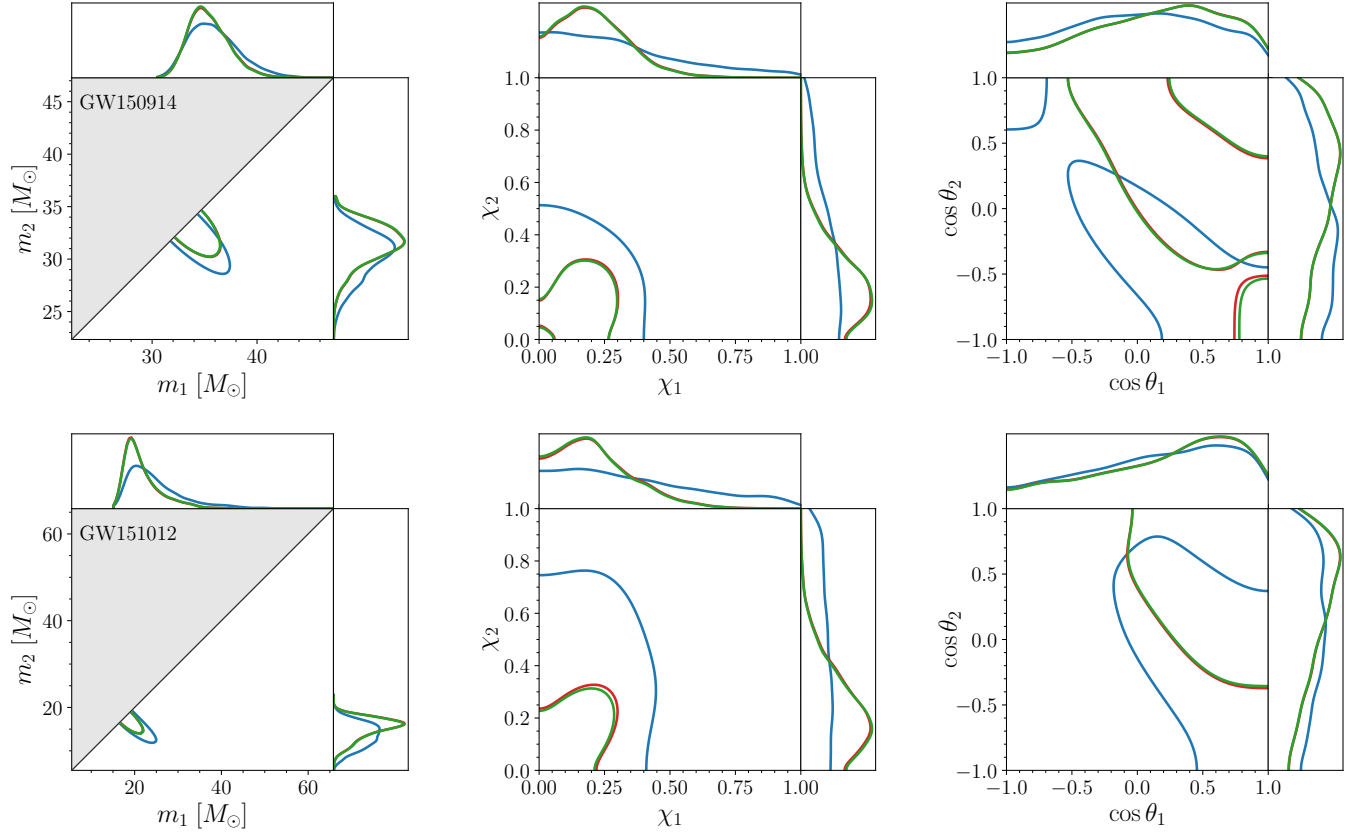

\* [moorecj@bham.ac.uk](mailto:moorecj@bham.ac.uk)

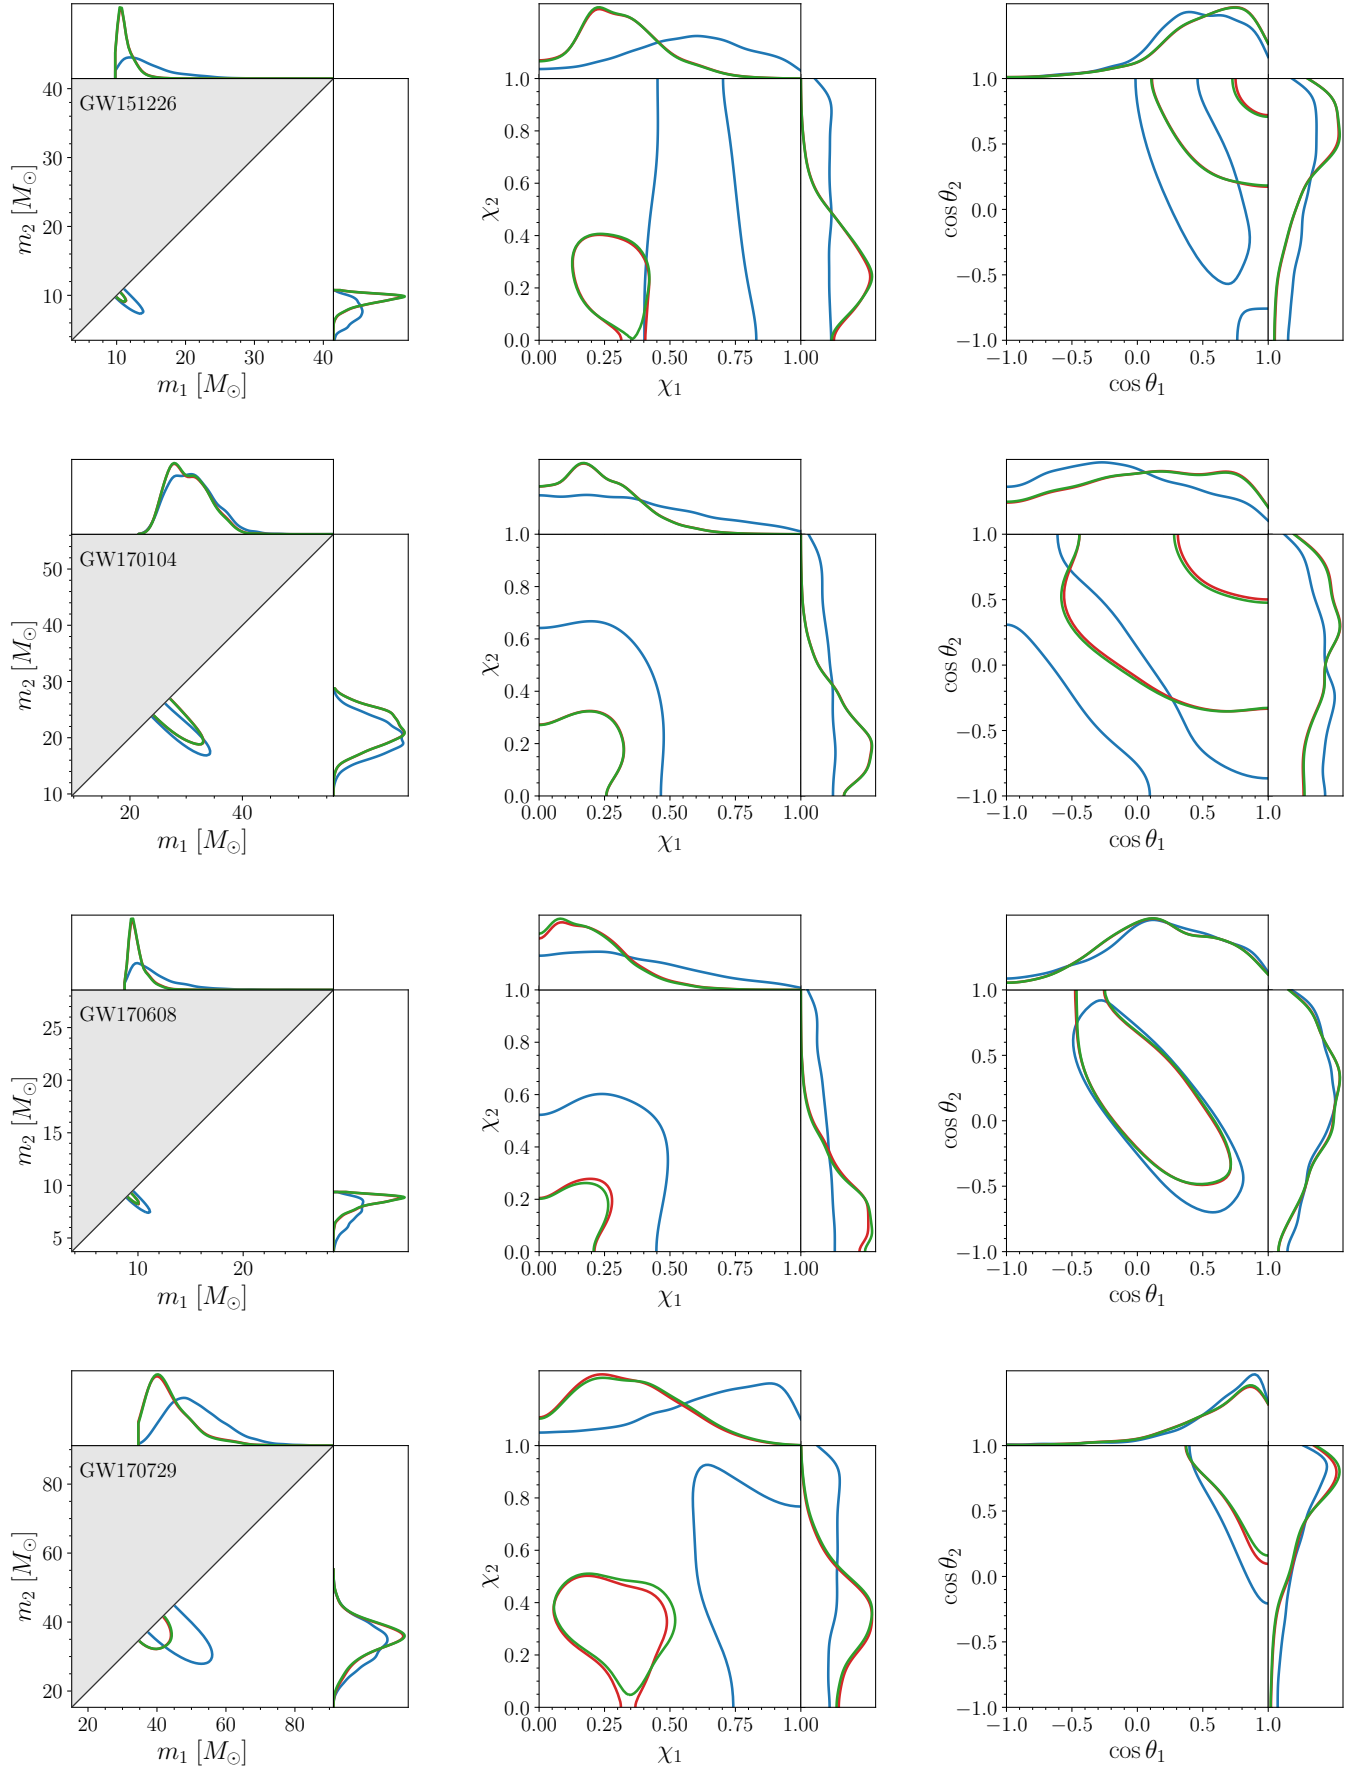

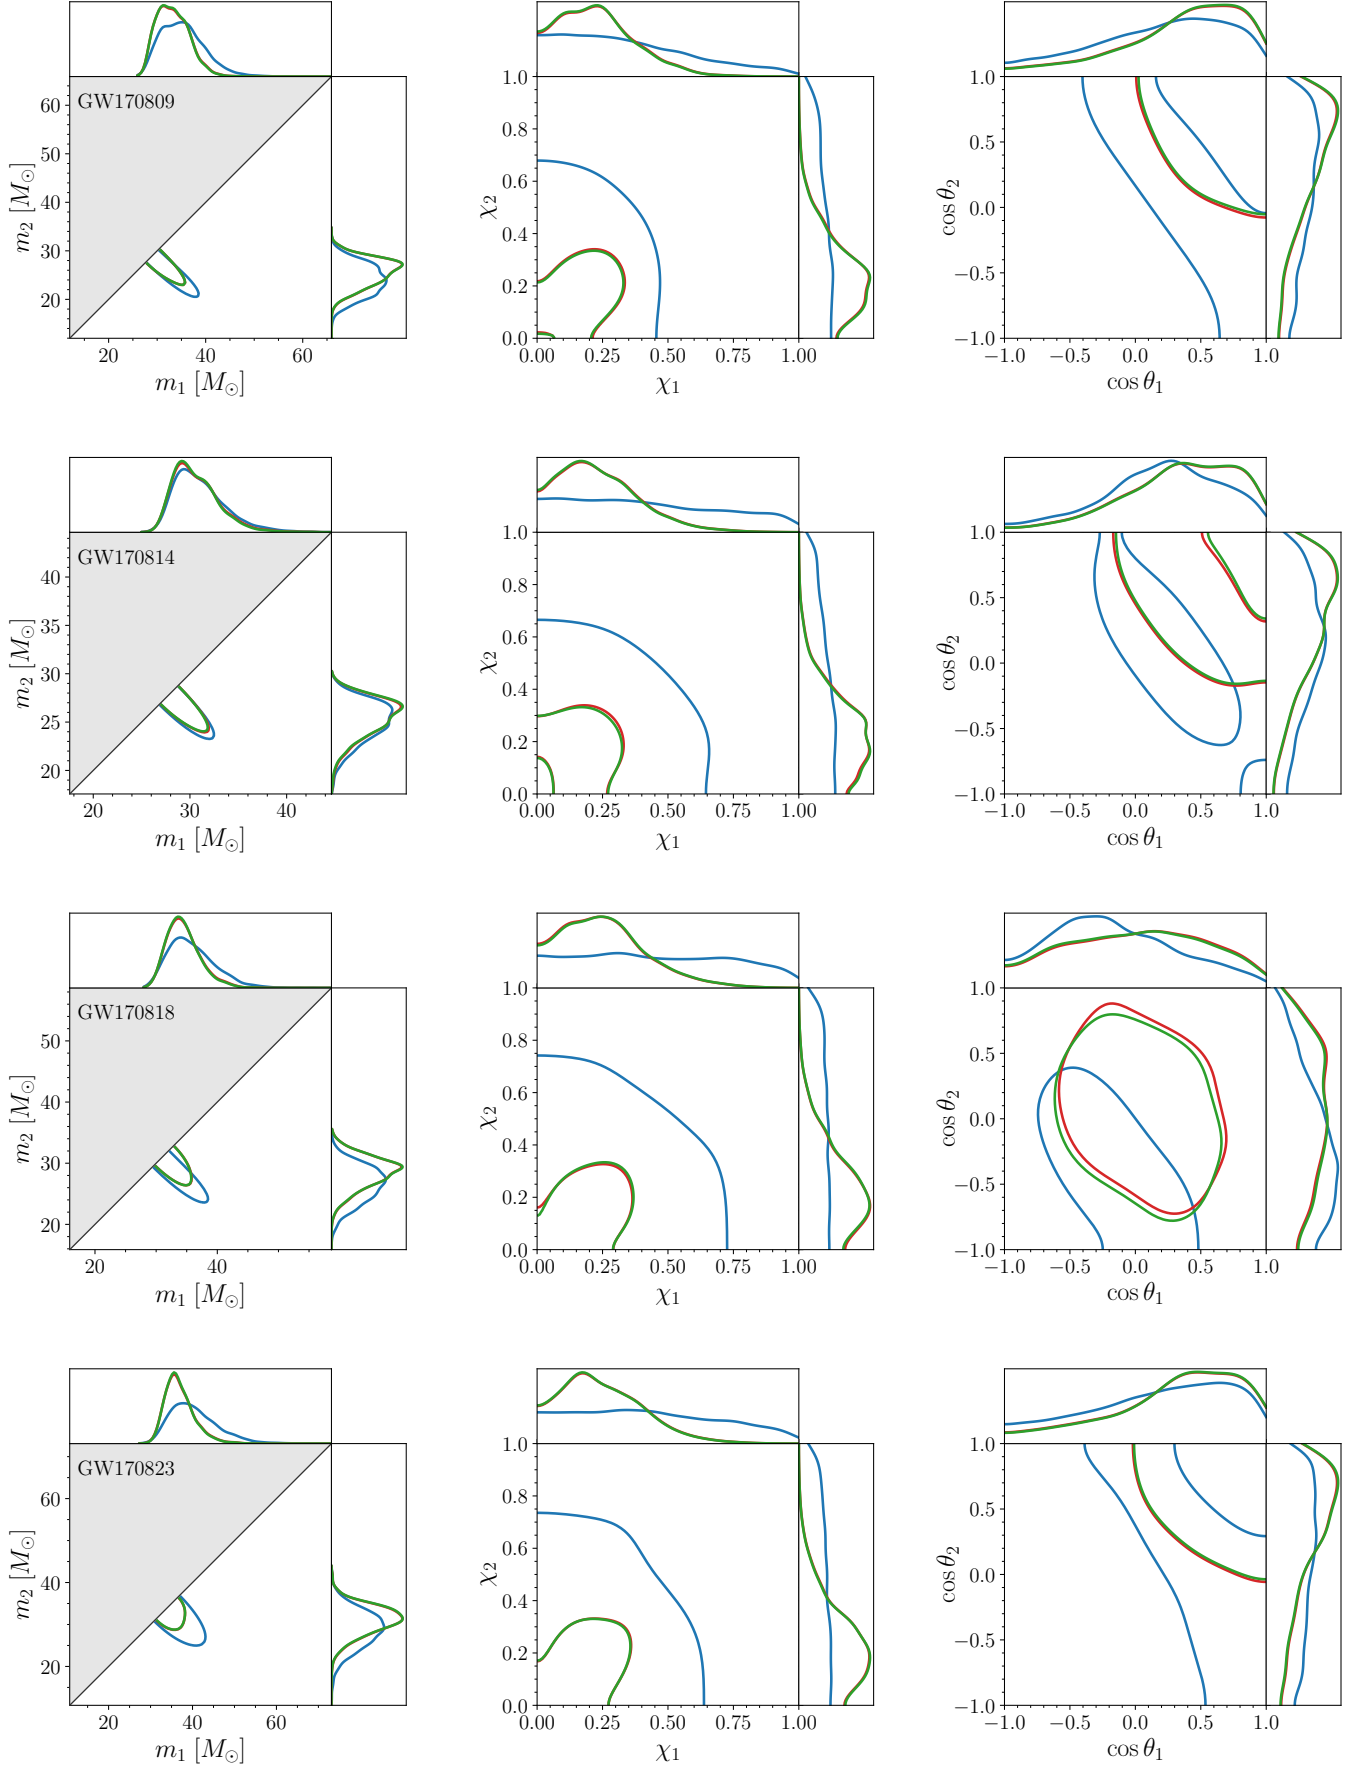

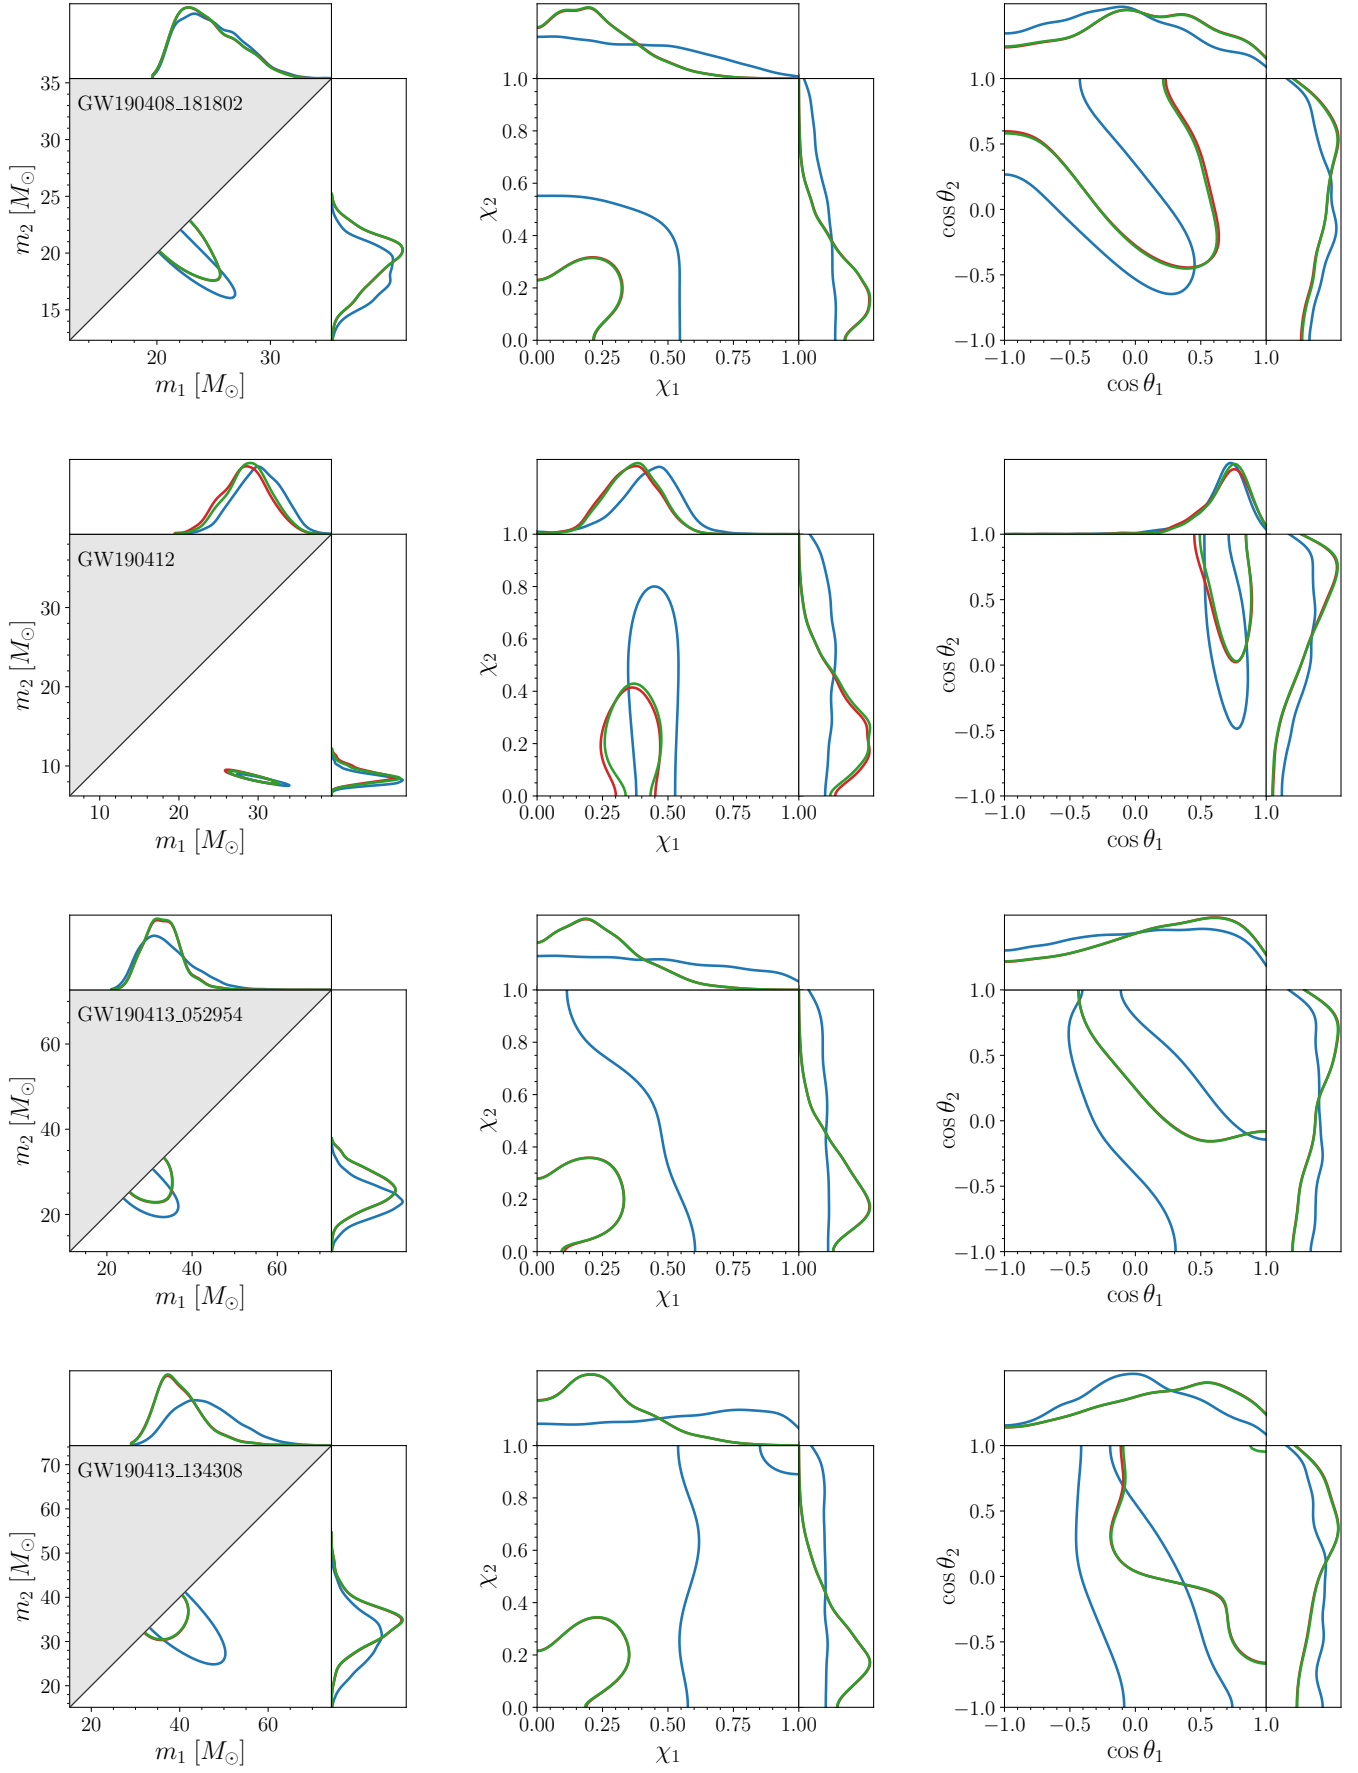

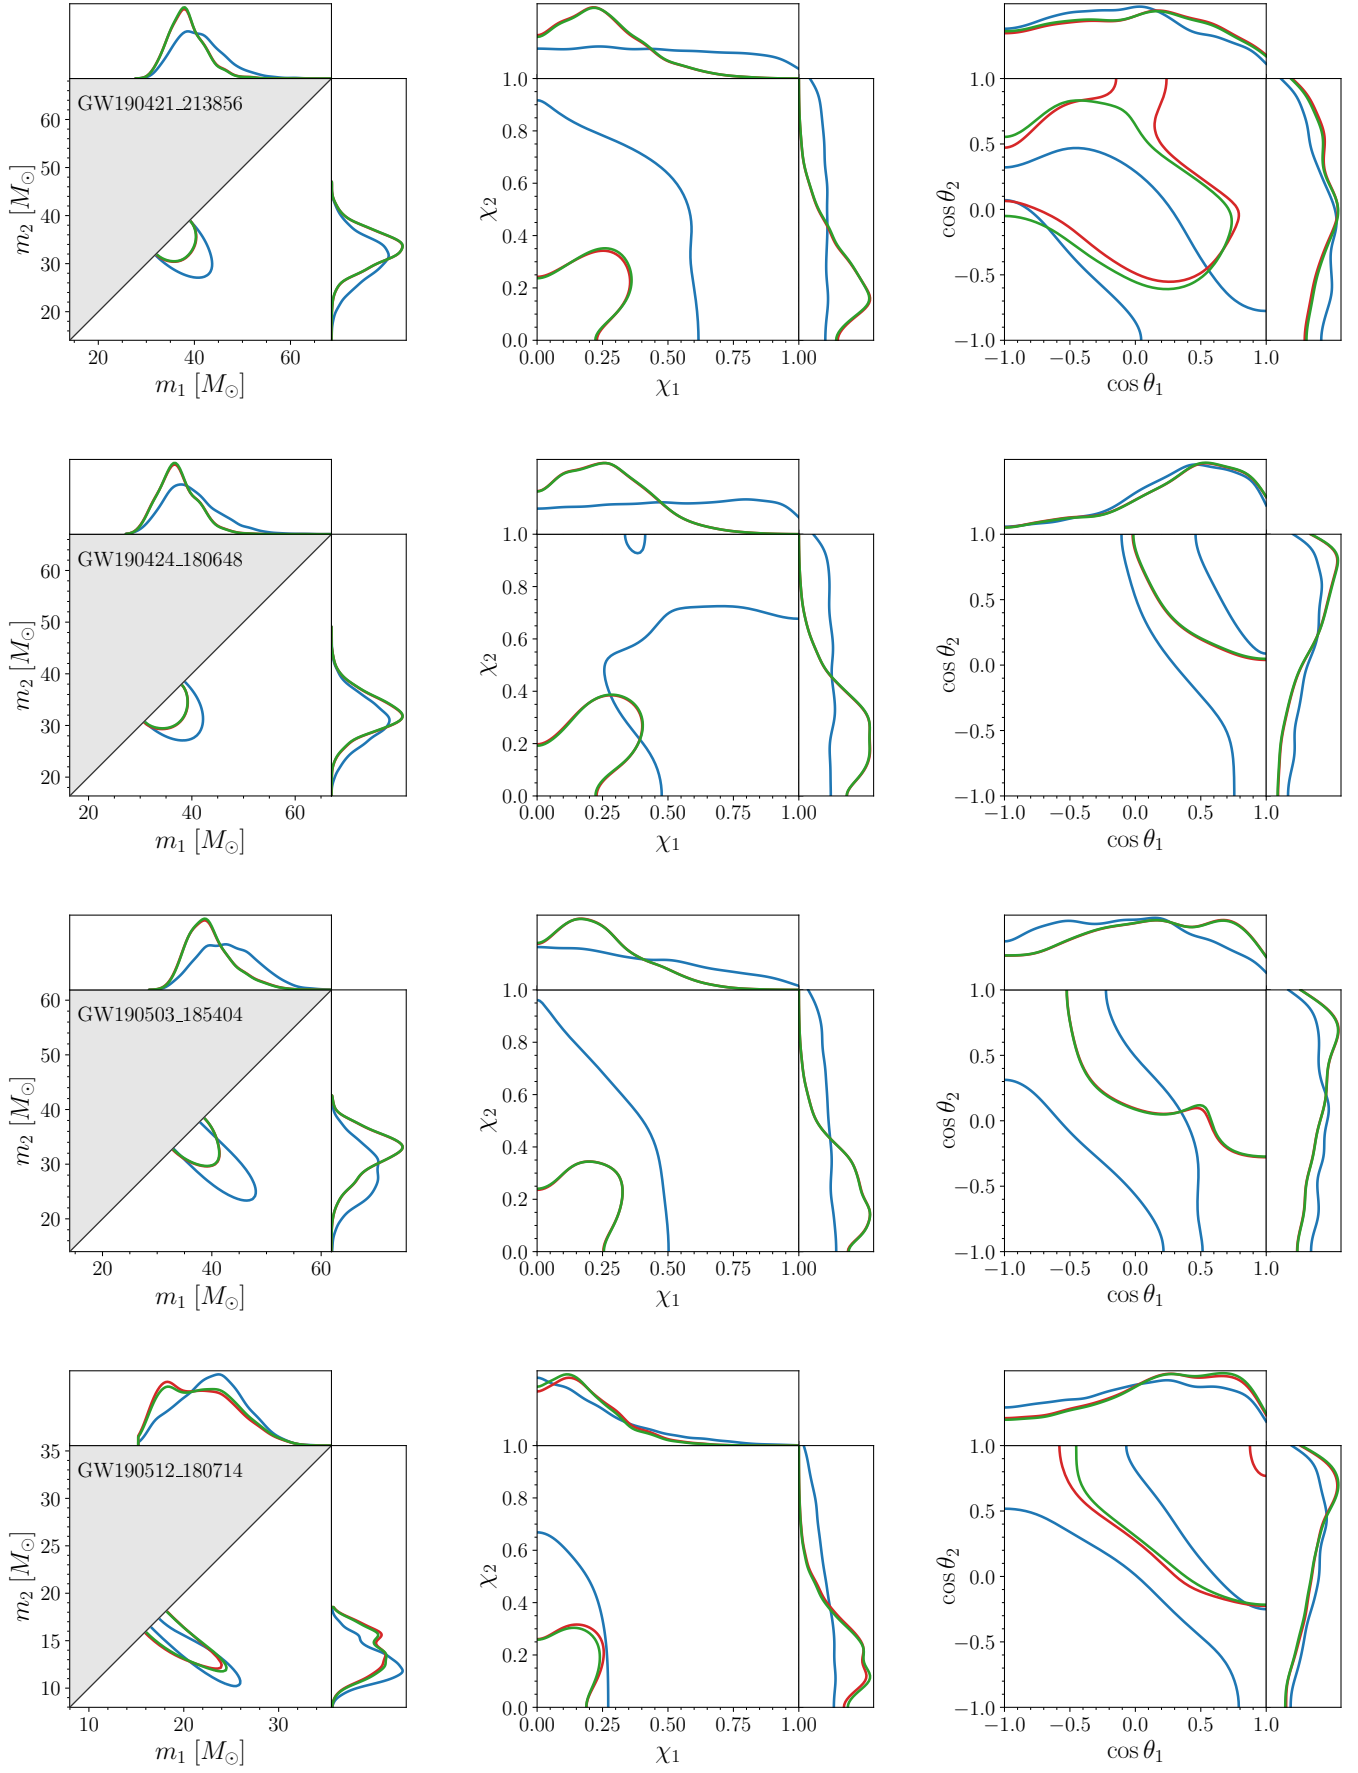

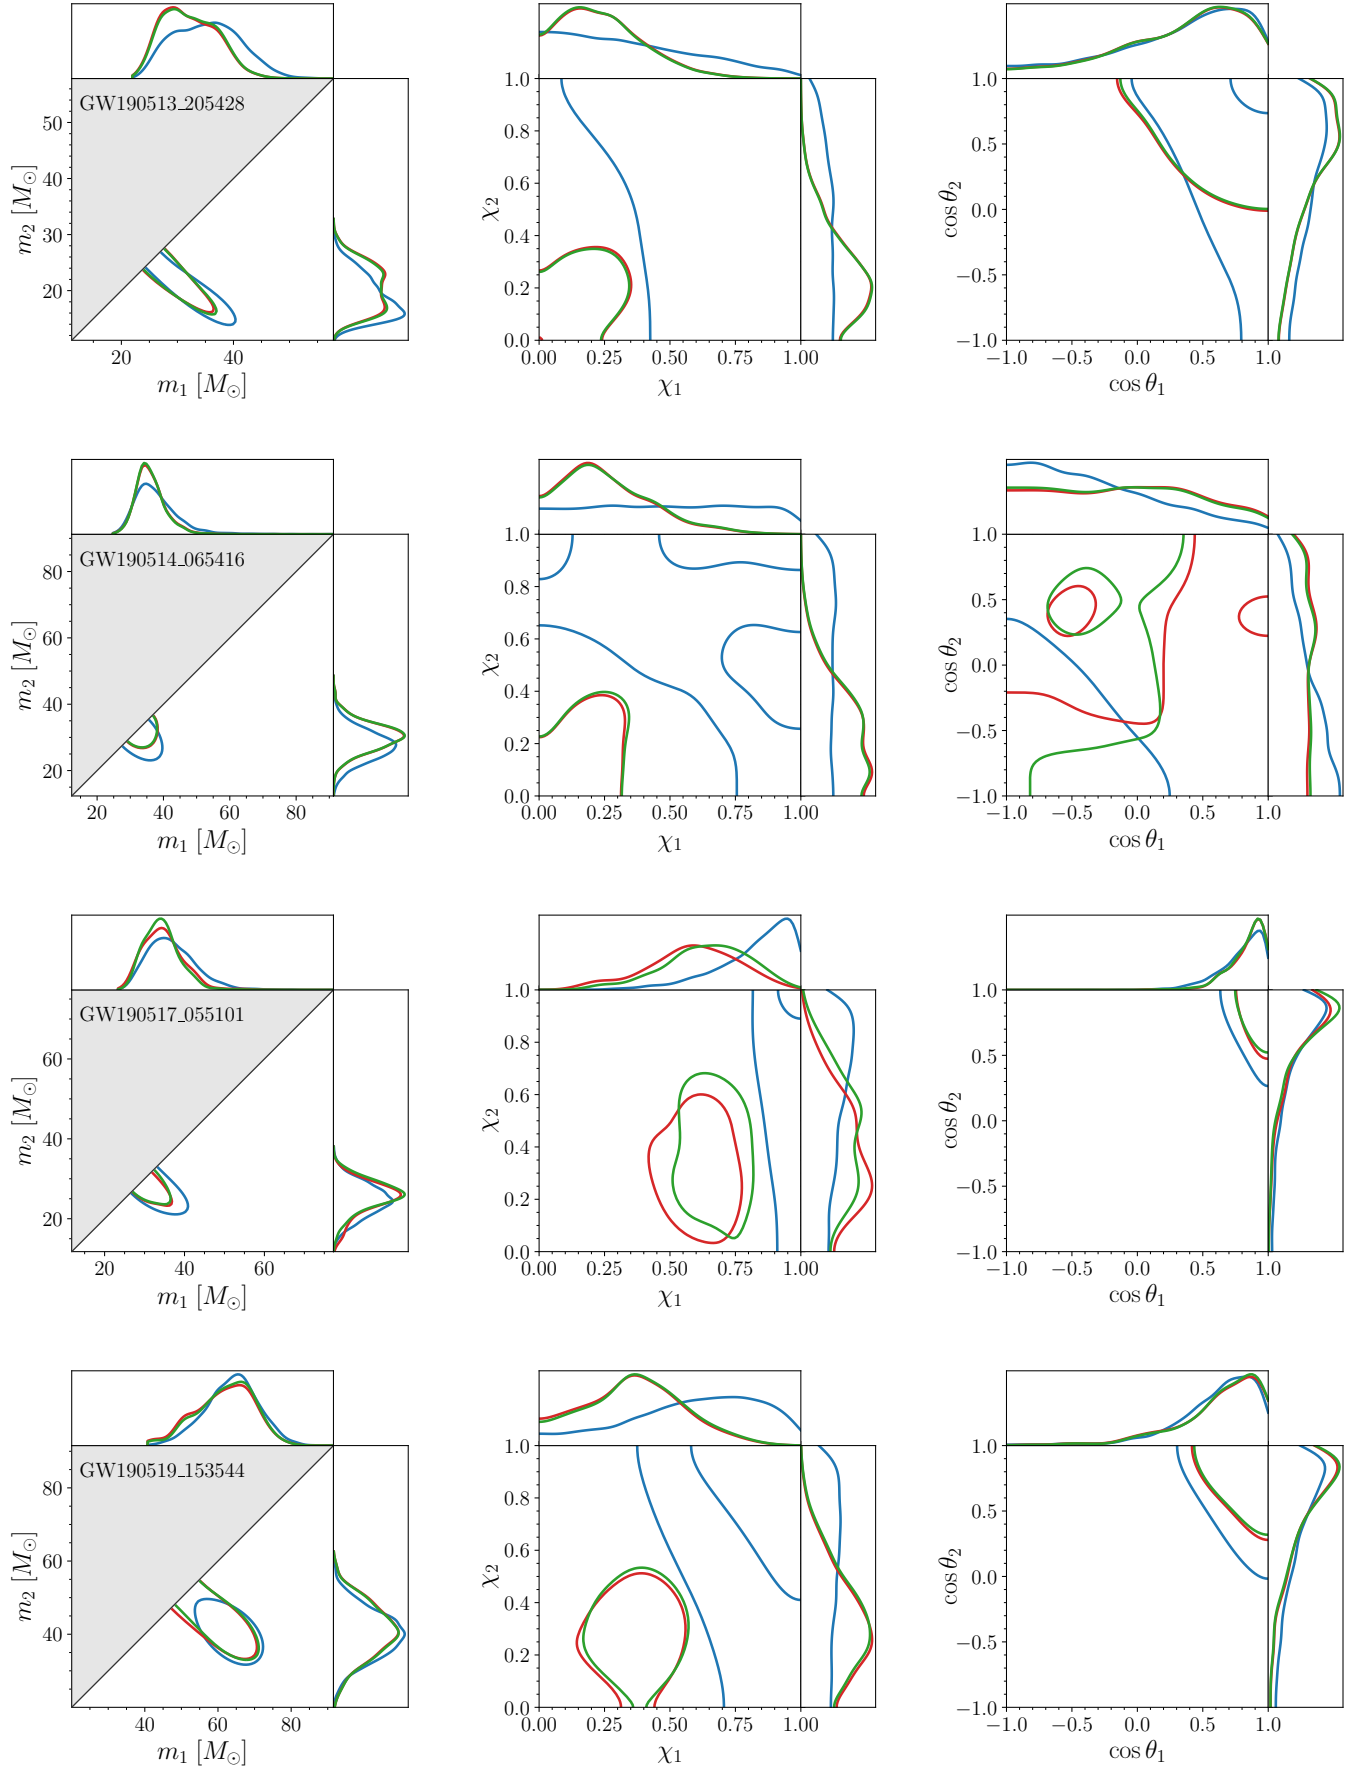

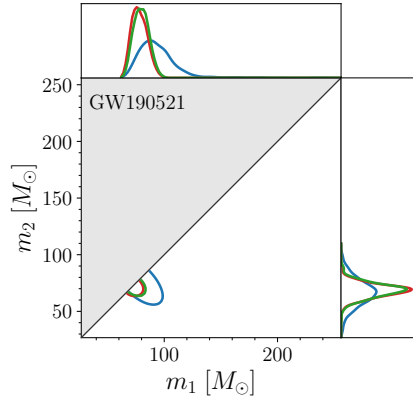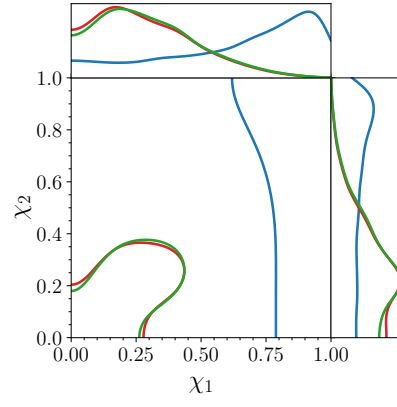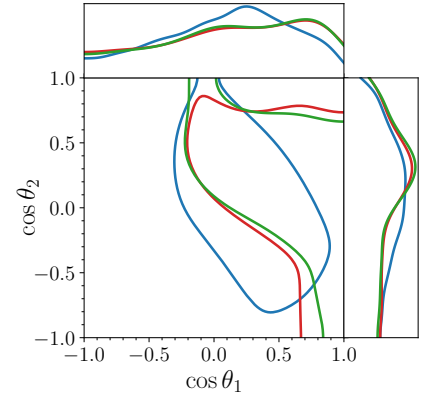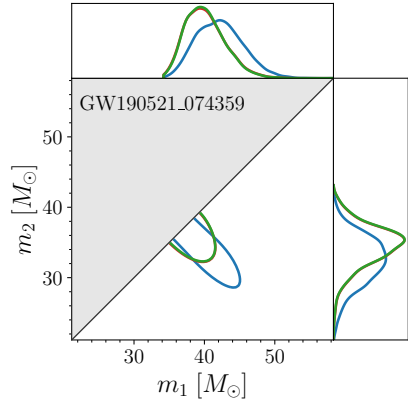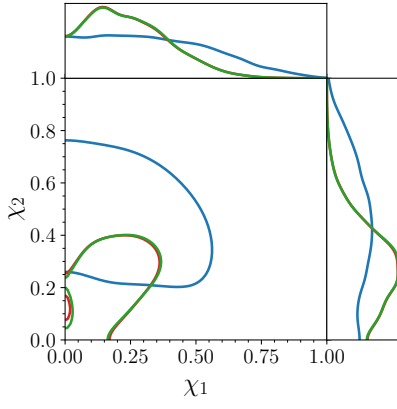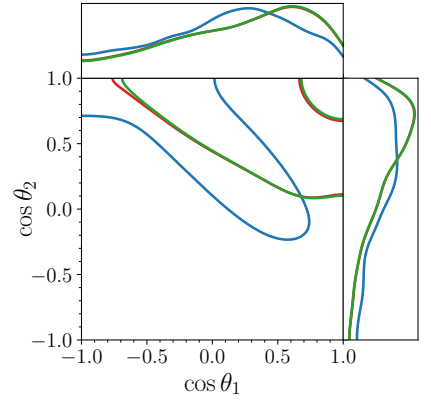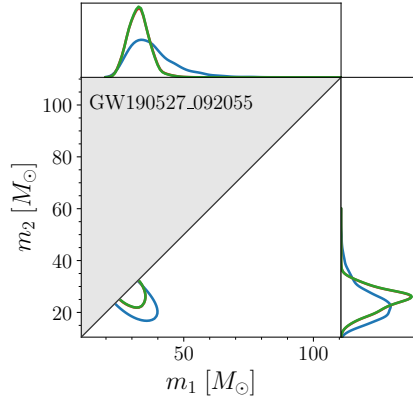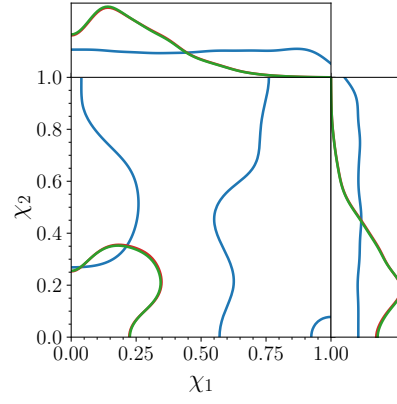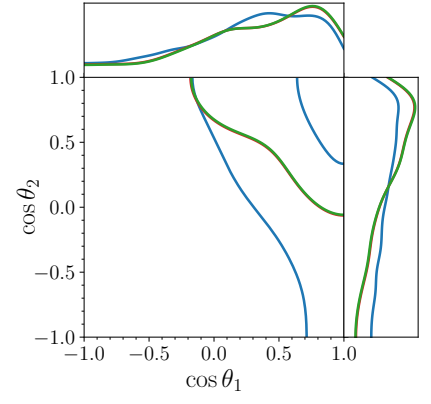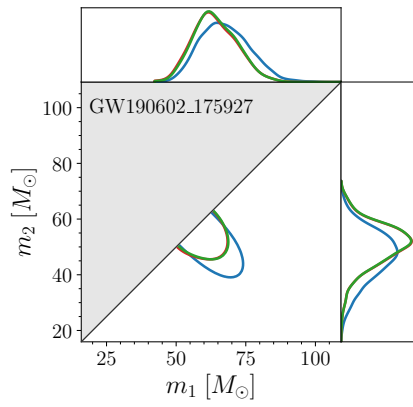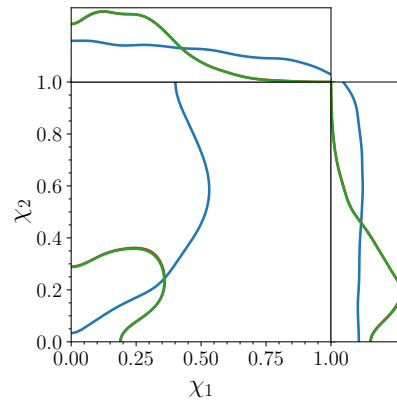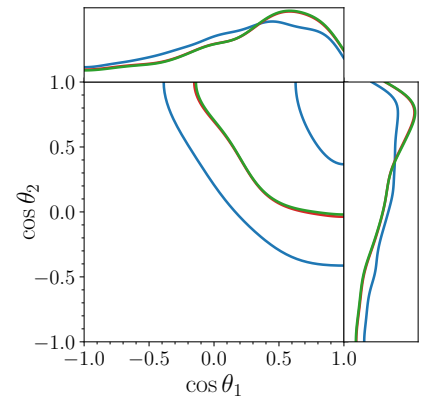

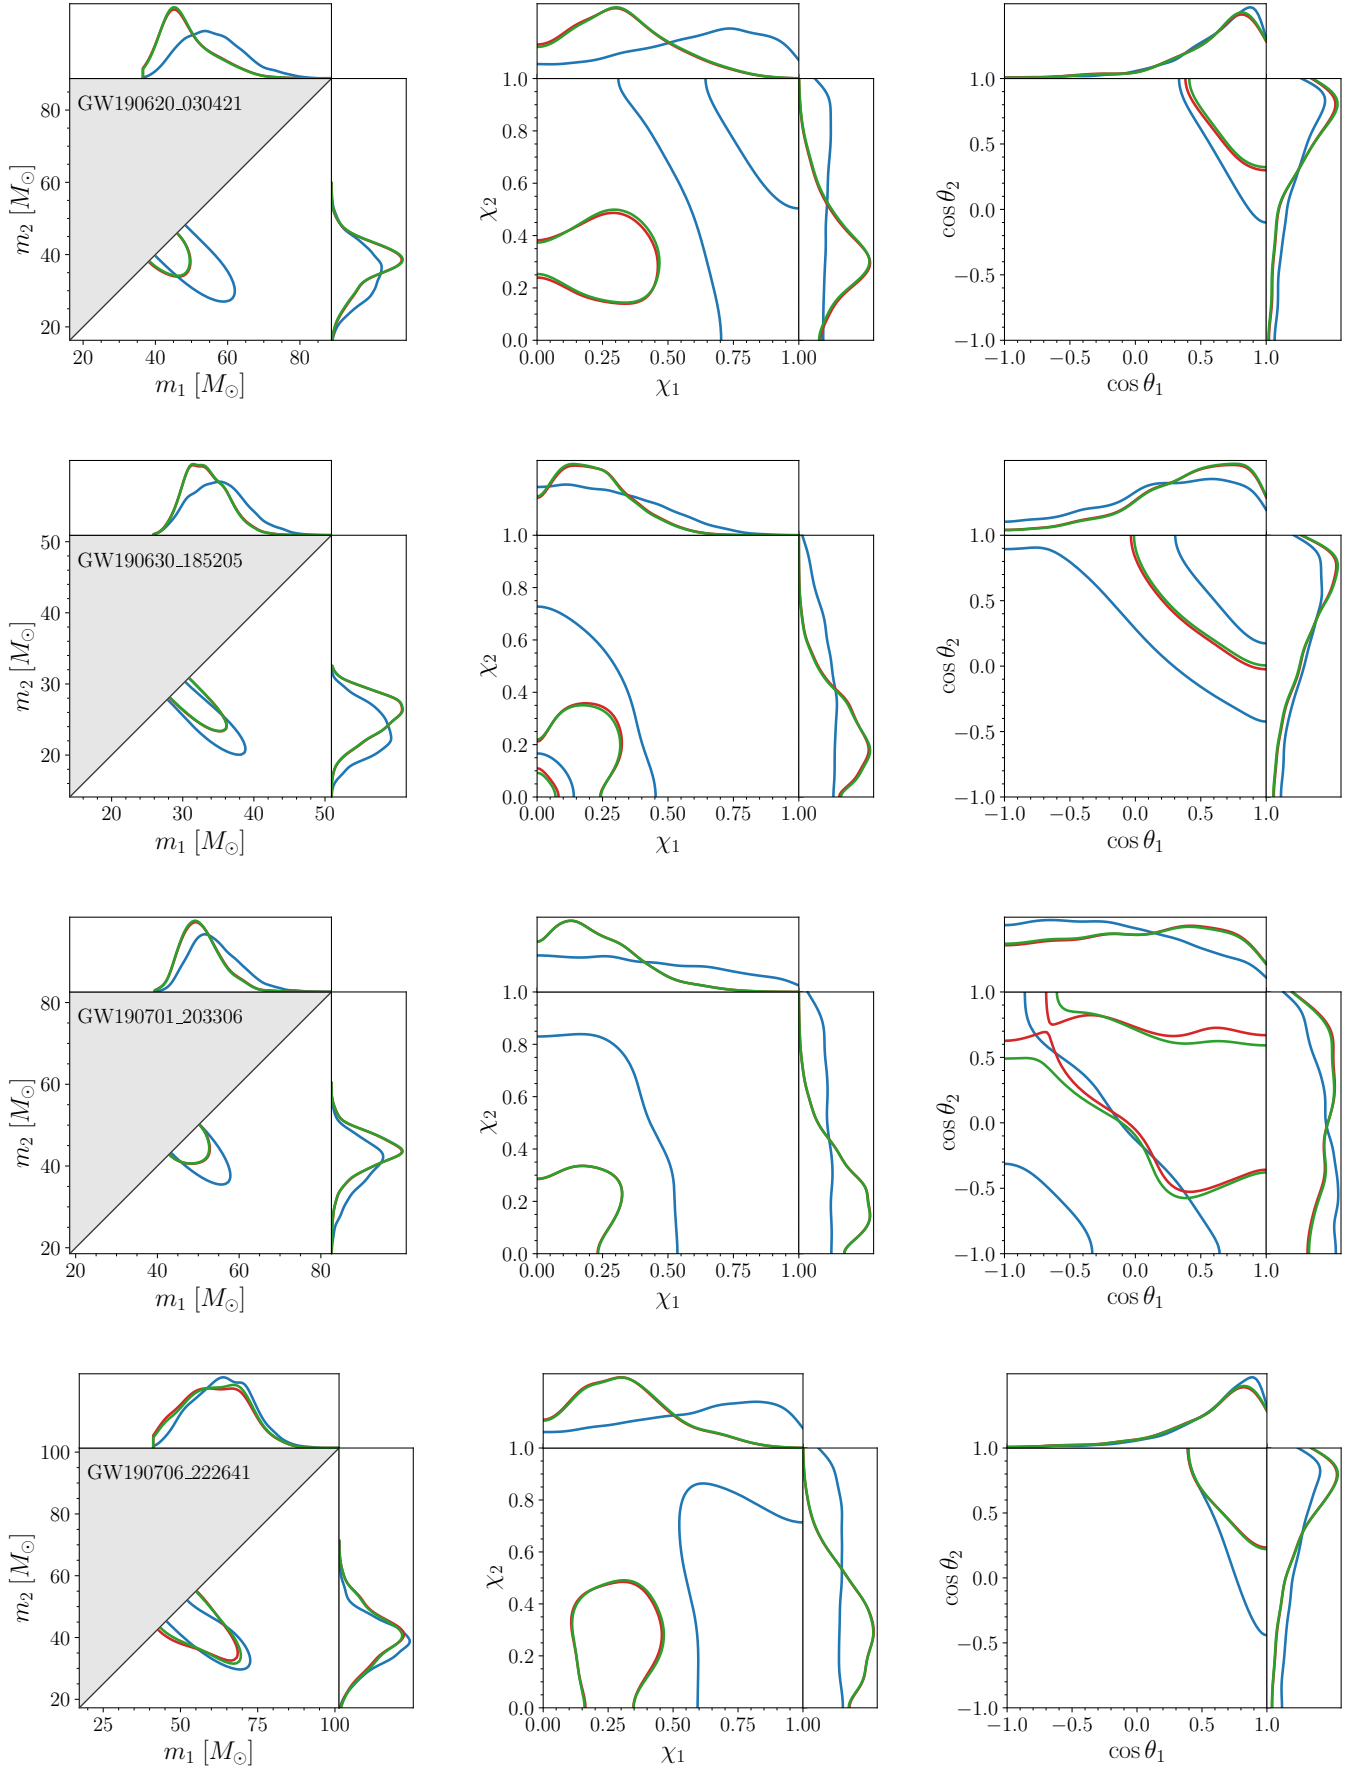

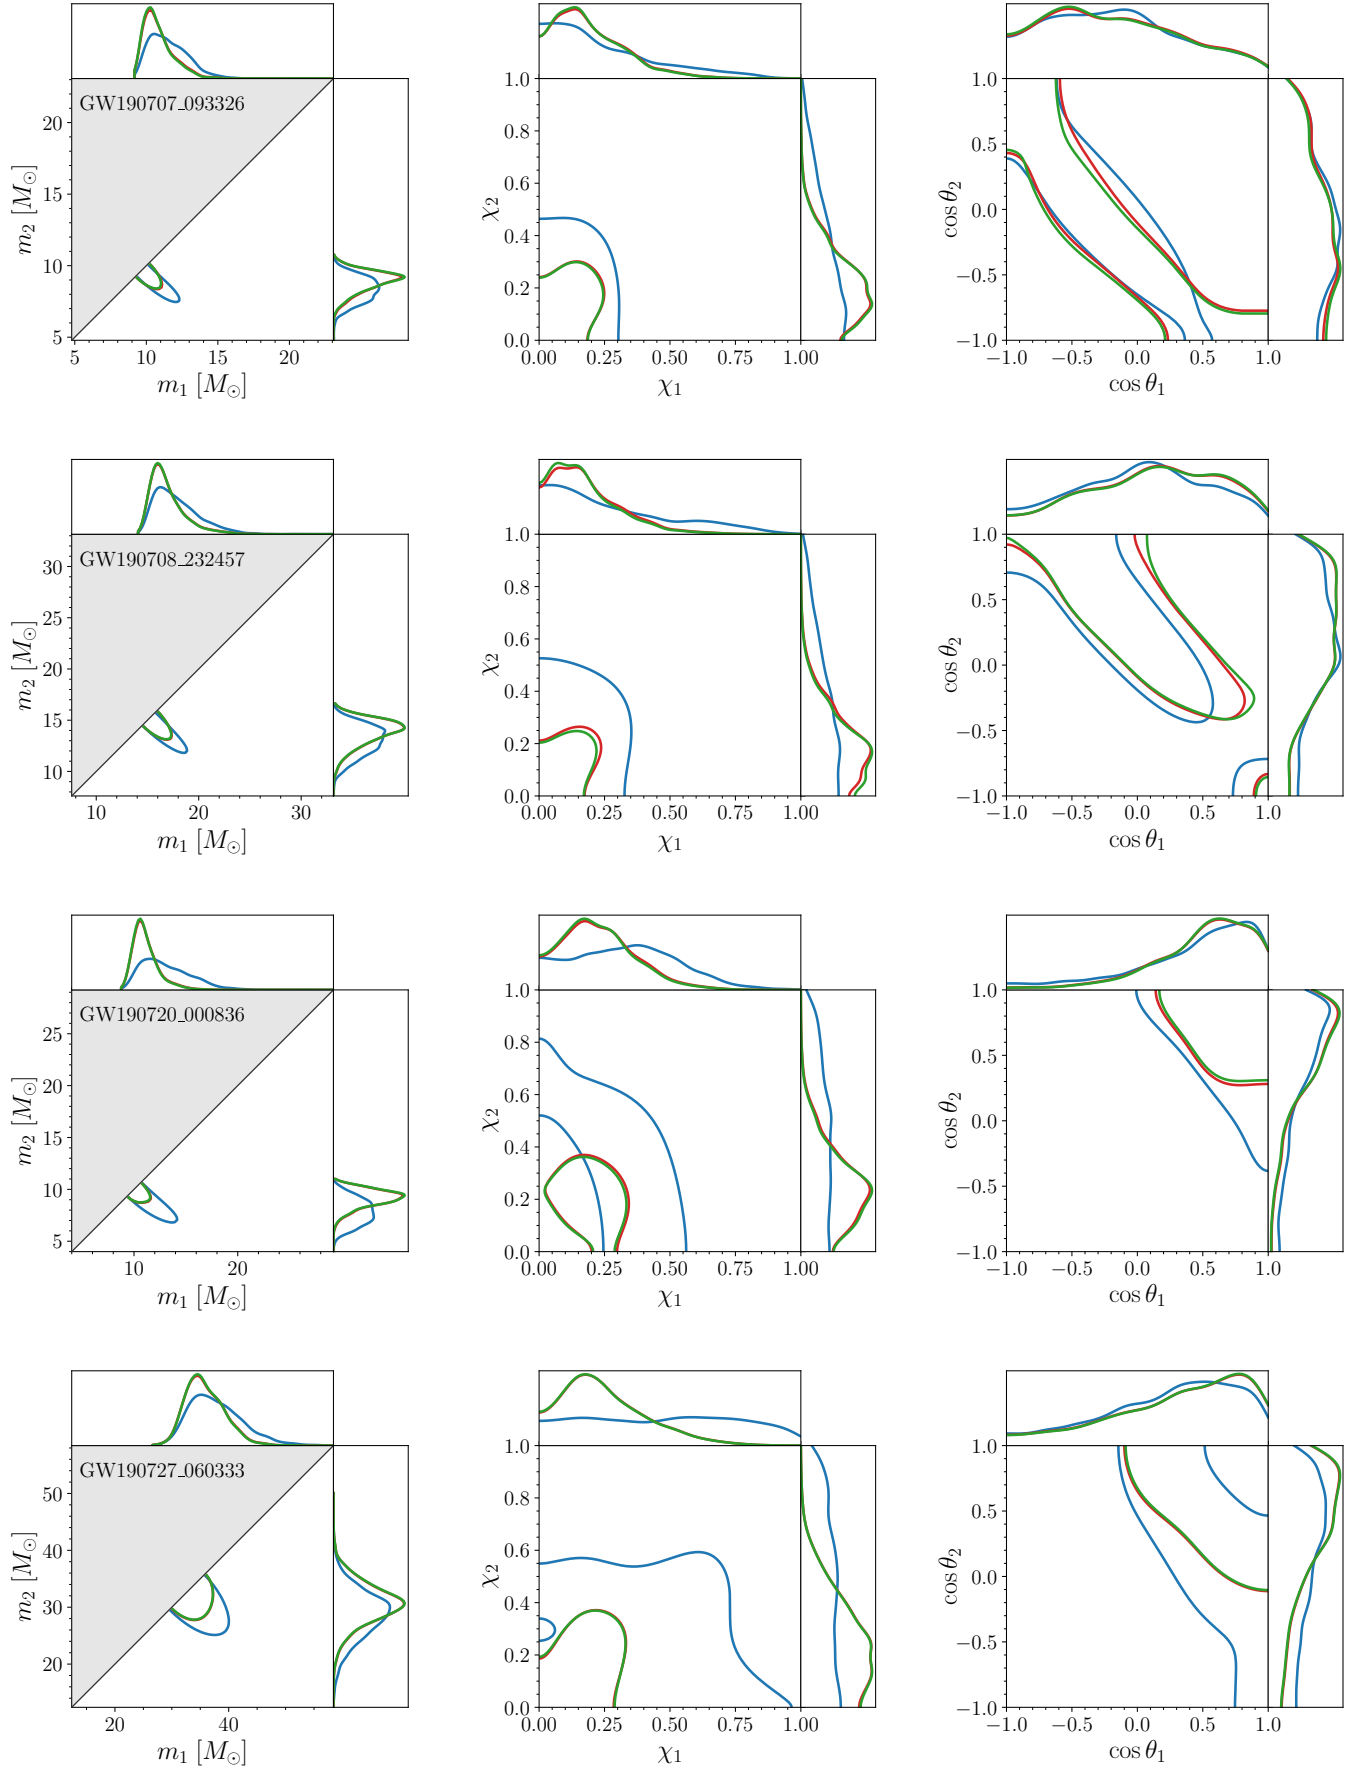

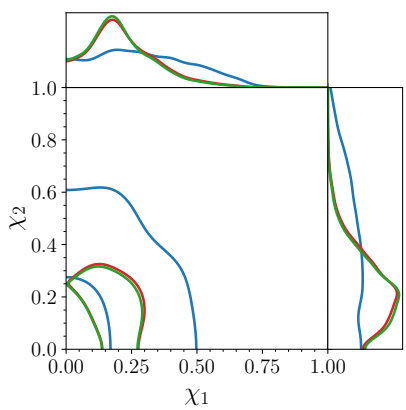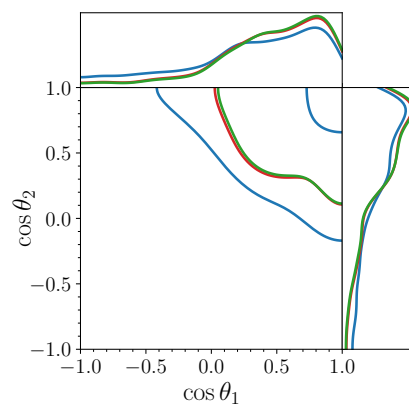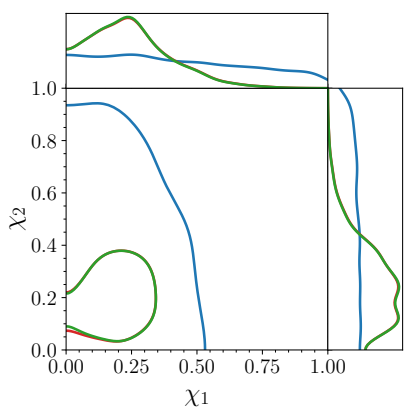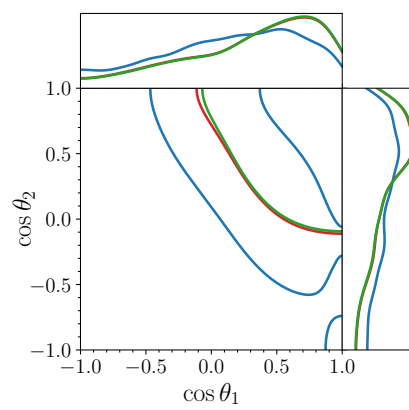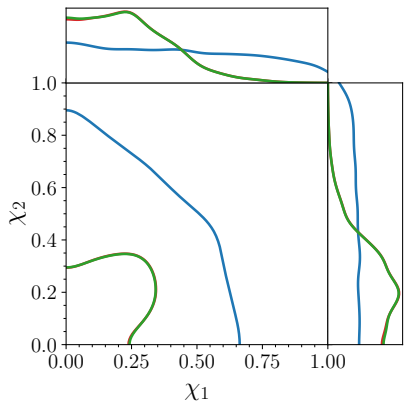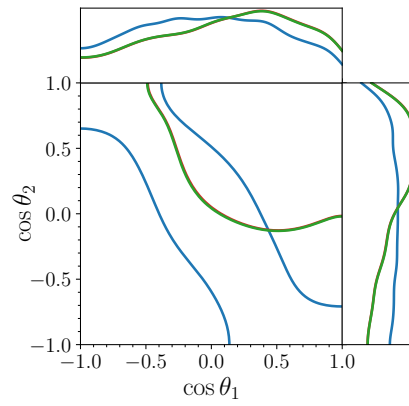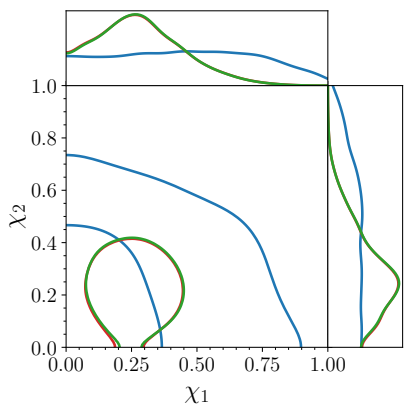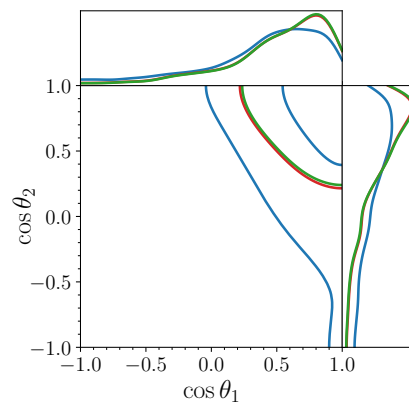

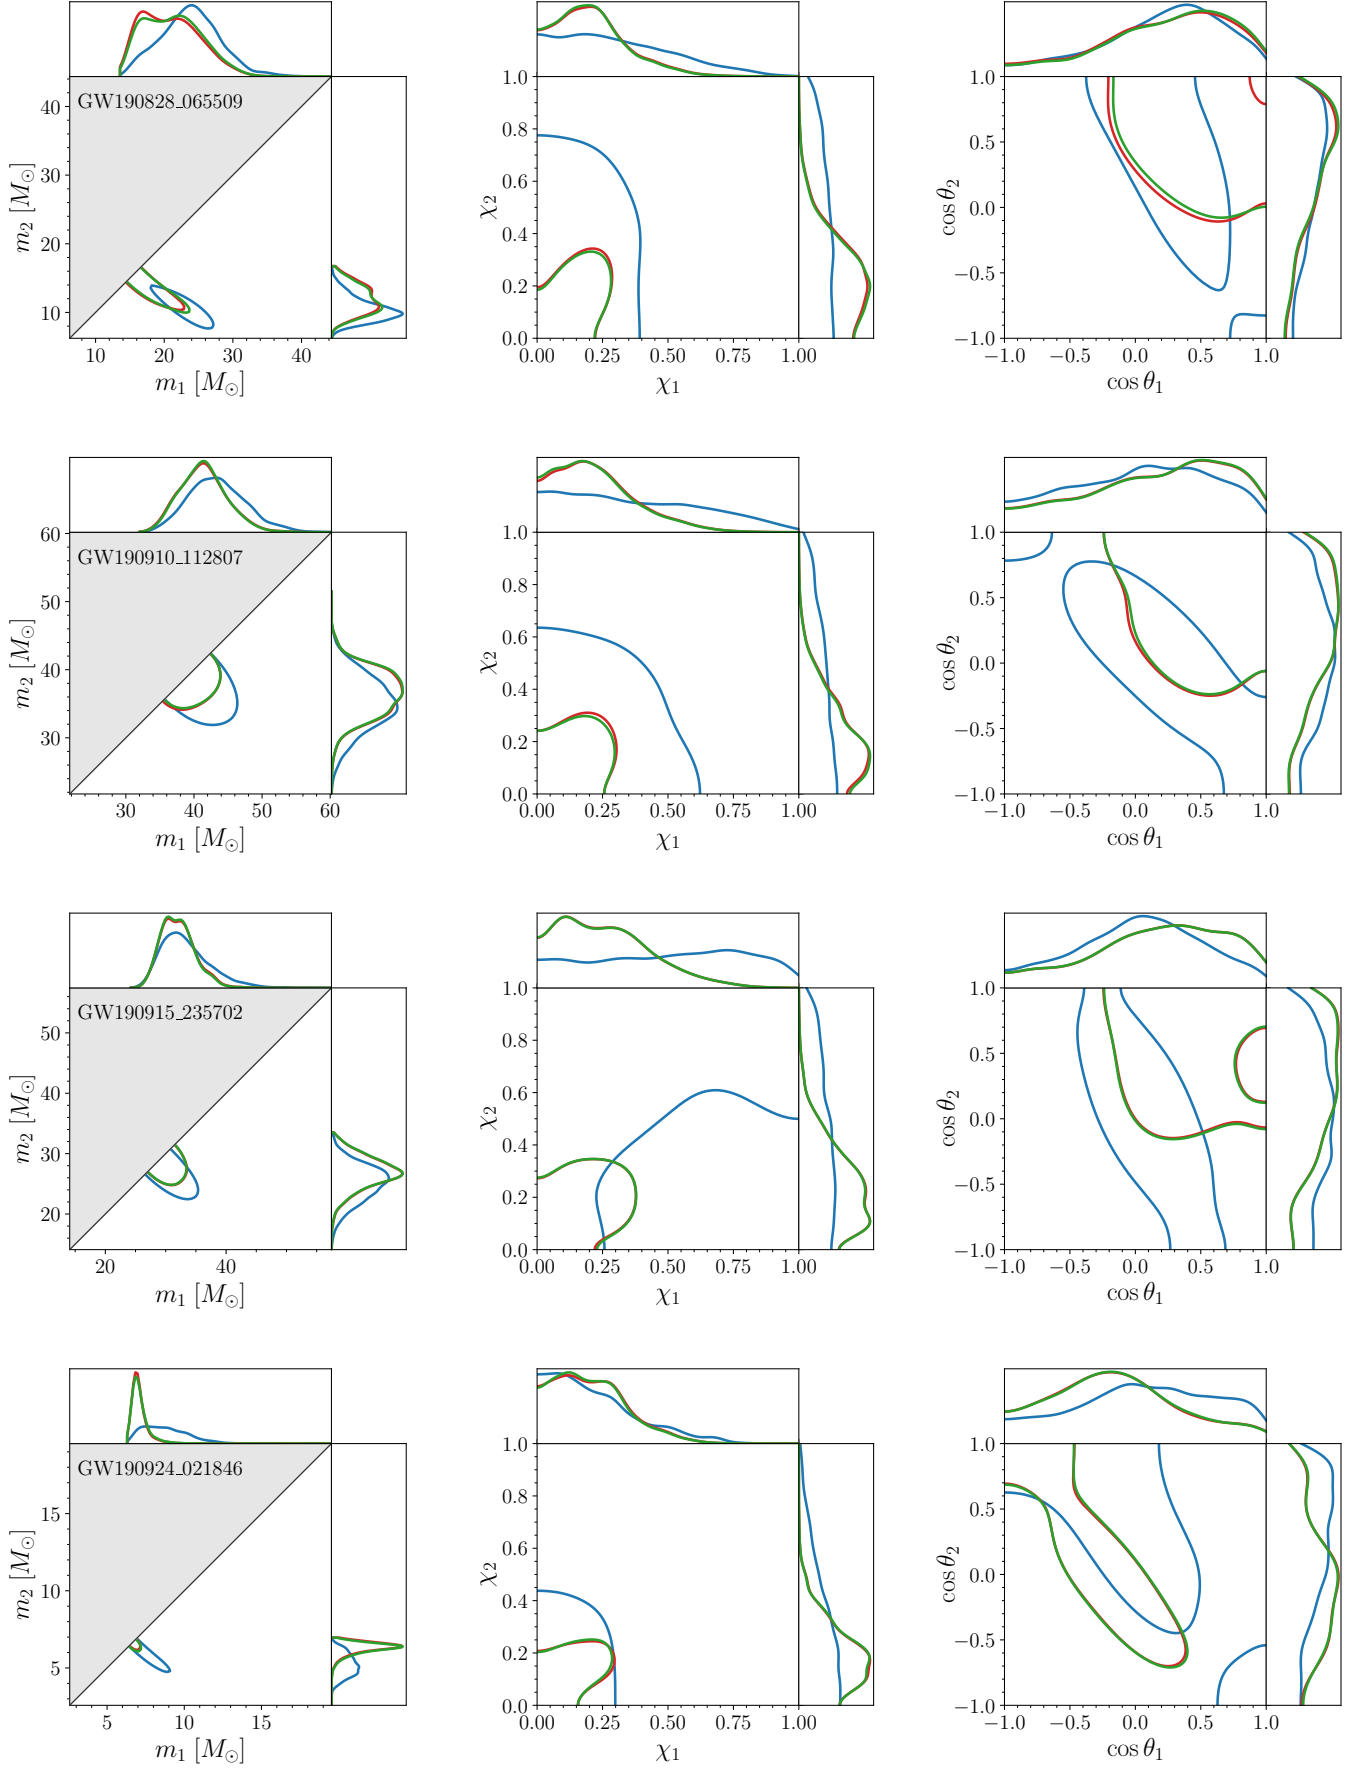

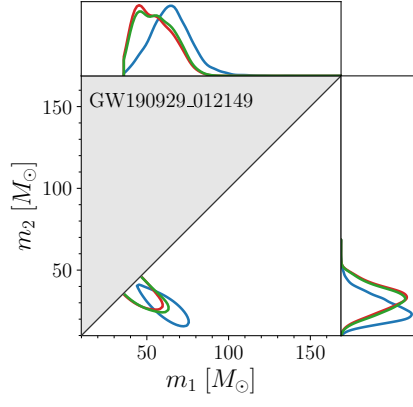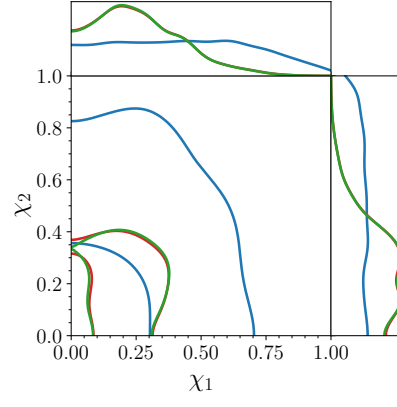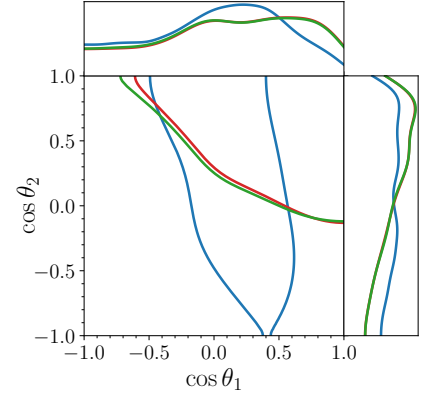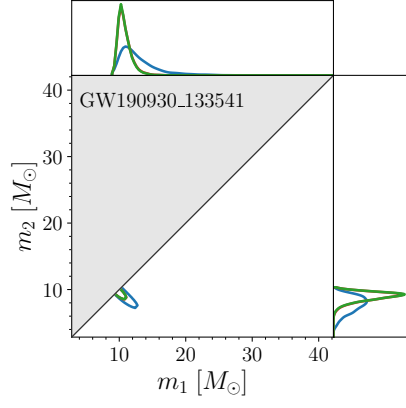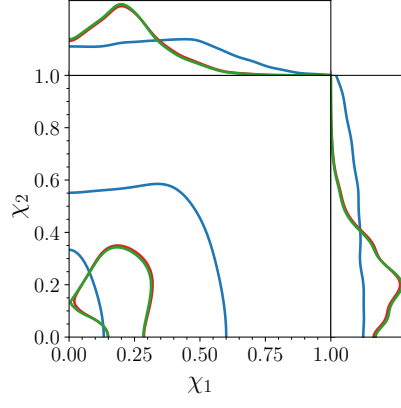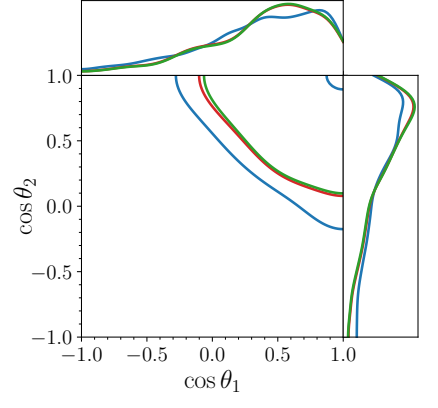

Supplement: Supplementary file 1 [file supp.pdf]
